# Supplementary material for: Extended Multi-Temperature Model for Electron--Phonon Coupling and Ultrafast Thermal Transport in Graphene
Source: arXiv:2511.22285 source file (2025-11-27)
Supplement: Supplementary file 1 [file Supplementary_Material.pdf]

# Supplementary Material: Extended Multi-Temperature Model for Electron–Phonon Coupling and Ultrafast Thermal Transport in Graphene

Houssem Rezgui*[1], Chuang Zhang†[2], and Clivia Sotomayor-Torres‡[1]

[1]INL – International Iberian Nanotechnology Laboratory, , Avenida Mestre José Veiga s/n, Braga 4715-330, Portugal
[2]Department of Physics, School of Sciences, , Hangzhou Dianzi University, Hangzhou 310018, China
[1]INL – International Iberian Nanotechnology Laboratory, Avenida Mestre José Veiga s/n, Braga 4715-330, Portugal
[2]Department of Physics, School of Sciences, Hangzhou Dianzi University, Hangzhou 310018, China

November 27, 2025

*houssem.rezgui@inl.int
†zhangc520@hdu.edu.cn
‡clivia.sotomayor@inl.int

This supplementary material outlines the governing equations of both approaches and provides a side-by-side comparison in terms of physical modeling, numerical implementation, and computational performance. The results highlight the trade-offs between accuracy, efficiency, and scalability, and justify the hybrid use of BTE and GKE solvers in future ultrafast transport modeling.

# 1 Governing equations

The governing equations presented here define the evolutions of the electron and phonon energy carriers in both the eMTM-BTE and eMTM-GKE frameworks. Each model incorporates multi-temperature dynamics, inter-subsystem coupling, and nonlocal transport behaviors, but they differ in mathematical formulation and computational complexity [1, 2]. The eMTM-BTE model is based on solving distribution functions derived from the Boltzmann transport equation under the discrete unified gas kinetic scheme (DUGKS) [3, 4]. It provides high-resolution predictions of energy density and heat flux in the phase space, suitable for materials where both ballistic and quasi-ballistic effects are significant.

$$\frac{\partial u_e}{\partial t} + \mathbf{v}_e \cdot \nabla u_e = \frac{u_e^{\mathrm{eq}} - u_e}{\tau_e} - \sum_i G_{ep,i}(T_e - T_{p,i}) \tag{S1}$$

$$\frac{\partial u_{p,i}}{\partial t} + \mathbf{v}_{p,i} \cdot \nabla u_{p,i} = \frac{u_{p,i}^{\mathrm{eq}} - u_{p,i}}{\tau_{p,i}} + G_{ep,i}(T_e - T_{p,i}) \tag{S2}$$

In the present kinetic simulation, $50 \times 100$ uniform cells are used to discretize the spatial domain in the $x-$ and $y-$ directions, respectively. 80 directions are used to equally discretize the two-dimensional solid angles, regardless of the system sizes. Time step is $\Delta t = 0.5$ fs and the grid independence tests clarify that the current numerical discretizations can meet the computational accuracy requirements.

The eMTM-GKE model simplifies transport by using a generalized thermal diffusion framework that employs partial differential equations (PDEs). It is derived from moment expansions of the BTE or directly from hydrodynamic

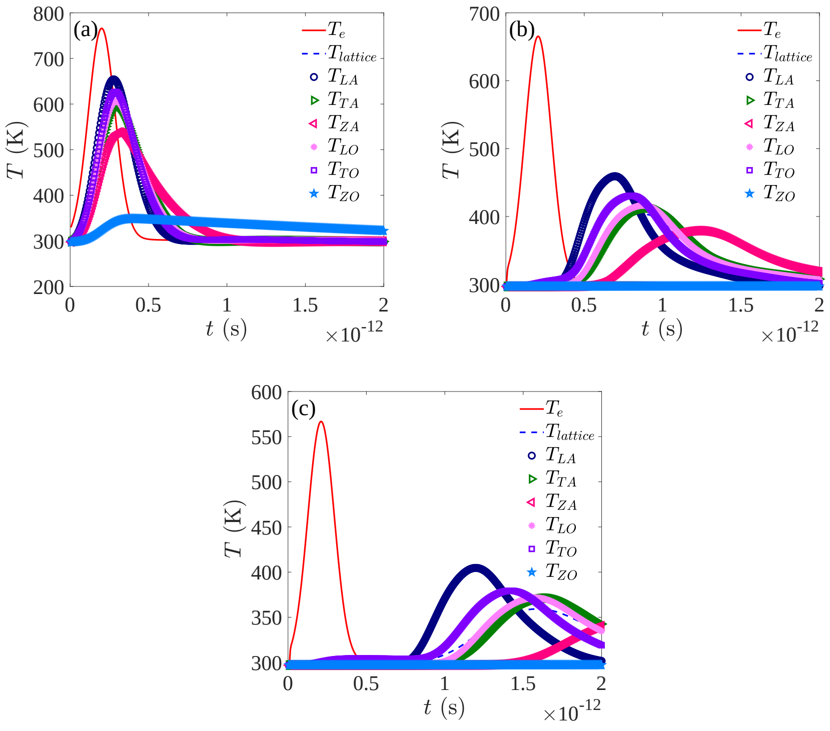


**Figure S1:** Temporal evolution of electron and phonon temperatures predicted by the eMTM-BTE model at different spatial positions. (a) $y = 1$ nm, (b) $y = 5$ nm and (c) $y = 10$ nm.

principles, capturing non-Fourier transport via second-order time derivatives and higher-order spatial gradients [5, 6, 7, 2].

$$\tau_e \frac{\partial^2 T_e}{\partial t^2} + \frac{\partial T_e}{\partial t} = \frac{\kappa_e}{C_e}\nabla^2 T_e + 3\ell_e^2 \nabla^2 \left(\frac{\partial T_e}{\partial t}\right) - \sum_i \frac{G_{ep,i}}{C_e}(T_e - T_{p,i}) \tag{S3}$$

$$\tau_{p,i} \frac{\partial^2 T_{p,i}}{\partial t^2} + \frac{\partial T_{p,i}}{\partial t} = \frac{\kappa_{p,i}}{C_{p,i}}\nabla^2 T_{p,i} + 3\ell_{p,i}^2 \nabla^2 \left(\frac{\partial T_{p,i}}{\partial t}\right) + \frac{G_{ep,i}}{C_{p,i}}(T_e - T_{p,i}) + \frac{G_{pp,i}}{C_{p,i}}(T_{\text{lat}} - T_{p,i}) \tag{S4}$$

For completeness, we present here the main expressions used to compute the branch-resolved effective thermal conductivity $k_{eff}$ from the multi-temperature framework. These equations follow directly from the solution of the eMTM-

BTE and eMTM-GKE models and account for the contributions of electrons and all relevant phonon branches. The formulation explicitly incorporates the size-dependent transport regime, enabling a seamless description of the ballistic-to-diffusive transition. The effective thermal conductivity of the electron and phonon branches is defined as the ratio of the heat flux carried by each branch to the corresponding temperature gradient along the same direction.

$$\kappa_{\text{eff},e} = \left| \frac{q_e L}{\Delta T} \right|, \tag{S5}$$

$$\kappa_{\text{eff},p,k} = \left| \frac{q_{p,k} L}{\Delta T} \right|, \tag{S6}$$

where $q_e$ and $q_{p,k}$ are the heat fluxes carried by electrons and the $k$-th phonon branch, respectively, $L$ is the transport length, and $\Delta T$ is the temperature difference across the system.

The eMTM-BTE model effectively captures the transient temperature evolution of all energy carriers at nanometer scales, as shown in Figure S1 (a), (b) and (c) for transport distances of $y = 1$ nm, $y = 5$ nm and $y = 10$ nm, respectively. The simulations reveal distinct temperature profiles for electrons and phonon branches, highlighting non-equilibrium dynamics and pronounced ballistic effects during the initial time regime. At $y = 1$ nm, the model predicts sharper temperature gradients and more significant deviations between subsystems, whereas at $y = 5$ nm and $y = 10$ nm, the results indicate enhanced energy exchange and partial thermalization. These findings underscore the capability of the eMTM-BTE framework to resolve highly localized, non-equilibrium heat transport phenomena. Figure S2 shows the temporal evolution of the electron temperature $T_e$ and $T_{LA}$ over a 2 ps window for eMTM-GKE and eMTM-BTE models. In both scenarios, Te exhibits a rapid initial decay while $T_{LA}$ rises correspondingly, indicating energy transfer from electrons to the lattice. The curves are qualitatively similar between $t_s = 95$ fs and $t_s = 110$ fs, suggesting that moderate changes in time step size have a minimal effect on the overall thermal dynamics in this range.

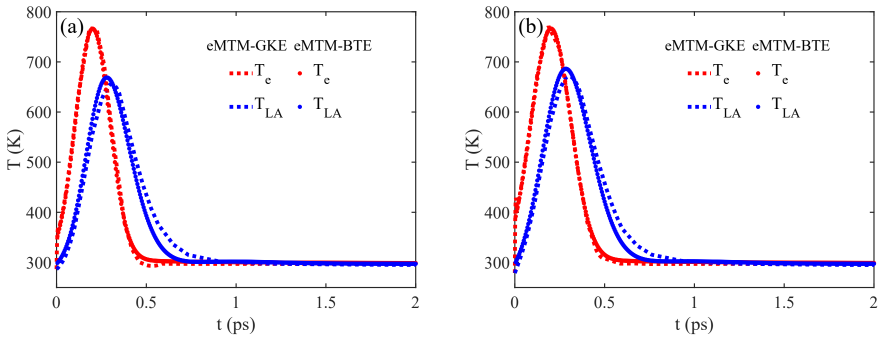


**Figure S2:** Temperature evolution of electron and ballistic phonon $LA$ mode predicted by the eMTM-BTE and eMTM-GKE models at $y = 1$ nm . (a) $t_s = 95$ fs, (b) $t_s = 110$ fs.

## 2 Model comparison and computational performance

This section compares the two extended models in terms of formulation, capability, and computational cost. The first Table (S1) outlines the conceptual and numerical differences between eMTM-BTE and eMTM-GKE. The second Table (S2) summarizes computational performance when simulating a 200 nm $\times$ 50 nm graphene domain under pulsed laser excitation.

Table S1. Comparison between eMTM-BTE and eMTM-GKE

| Feature | eMTM-BTE | eMTM-GKE |
|---|---|---|
| Model | BTE | Extended GKE |
| Physical basis | Kinetic theory | Continuum approximation |
| Transport regime | Ballistic to diffusive | Ballistic to diffusive |
| Nonlocal effects | Directly resolved | Modeled via higher-order terms |
| Temporal accuracy | High (distribution-level) | Moderate (thermal fields) |
| Numerical scheme | DUGKS | Finite element method |

Table S2. Computational performance for a 200 × 50 nm graphene system

| Metric | eMTM-BTE | eMTM-GKE |
| --- | --- | --- |
| Equations solved | 7 BTEs (1 e + 6 ph) | 7 PDEs (temperatures) |
| Time step | 0.5 fs | 1 fs |
| Total time simulated | 2 ps | 2 ps |
| CPU runtime | 96 seconds (40 cores) | 15 minutes (14 cores) |
| Suitability | Fast, accurate | Fast, accurate |

Figure S3 shows the conceptual framework underlying the two extended MTM models, illustrating their fundamentally different approaches to describing multi-carrier heat transport in nanoscale materials. The BTE approach treats transport phenomena through a particle-based kinetic theory framework, where discrete carriers—electrons (red), longitudinal acoustic phonons (green), longitudinal optical phonons (blue), and out-of-plane acoustic phonons (purple)—are individually tracked with their associated trajectories, enabling the direct resolution of ballistic-to-diffusive transport regimes with high temporal accuracy. In contrast, the GKE approach employs a continuum approximation where these same energy carriers are represented as temperature fields (Te, TLA, TLO, TZA) with diffusive gradients, capturing non-local and memory effects through higher-order partial differential equations rather than explicit particle tracking. This visual comparison highlights why the BTE method requires the sophisticated DUGKS solver for managing particle-based calculations in velocity-position space, while the GKE approach utilizes a conventional finite element scheme to solve the coupled temperature field equations, ultimately leading to the computational performance differences reported in Table S2.

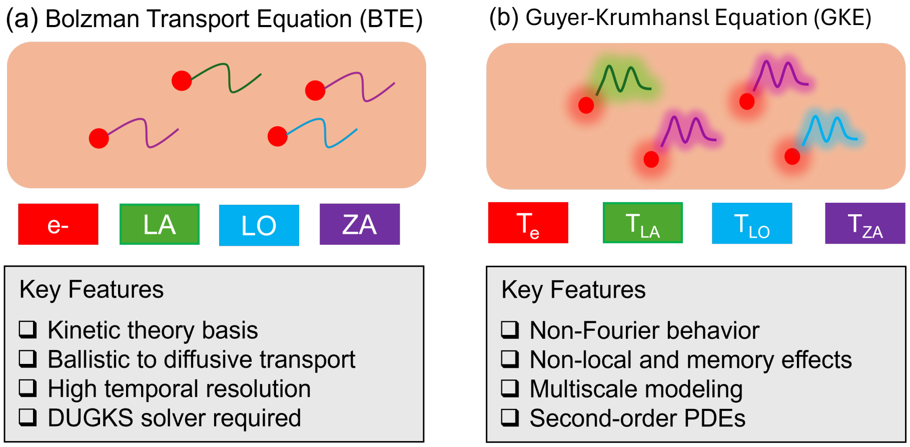


**Figure S3:** Conceptual framework comparison of (a) eMTM-BTE approach with discrete carriers and trajectories, and (b) eMTM-GKE approach with temperature field representations for multi-carrier heat transport modeling.

## References

[1] Z. Lu, A. Vallabhaneni, B. Cao, X. Ruan, Phonon branch-resolved electron-phonon coupling and the multitemperature model, Phys. Rev. B 98 (2018) 134309. URL: https://link.aps.org/doi/10.1103/PhysRevB.98.134309. doi:10.1103/PhysRevB.98.134309.

[2] M. Habibi, A. Beardo, L. Cui, Near-field thermal radiation as a probe of nanoscale hot electron and phonon transport, ACS Nano 19 (2025) 6033–6043. URL: https://doi.org/10.1021/acsnano.4c11893. doi:10.1021/acsnano.4c11893.

[3] C. Zhang, H. Rezgui, M. Lian, H. Liang, Non-equilibrium transport and phonon branch-resolved size effects based on a multi-temperature kinetic model, arXiv:2505.02411 (2025). URL: https://arxiv.org/abs/2505.02411. doi:https://doi.org/10.48550/arXiv.2505.02411.

[4] C. Zhang, R. Guo, M. Lian, J. Shiomi, Electron–phonon coupling

and non-equilibrium thermal conduction in ultra-fast heating systems, Applied Thermal Engineering 249 (2024) 123379. URL: https://www.sciencedirect.com/science/article/pii/S1359431124010470. doi:https://doi.org/10.1016/j.applthermaleng.2024.123379.

[5] R. A. Guyer, J. A. Krumhansl, Solution of the linearized phonon boltzmann equation, Phys. Rev. 148 (1966) 766–778. URL: https://link.aps.org/doi/10.1103/PhysRev.148.766. doi:10.1103/PhysRev.148.766.

[6] H. Rezgui, Phonon hydrodynamic transport: Observation of thermal wave-like flow and second sound propagation in graphene at 100 k, ACS Omega 8 (2023) 23964–23974. URL: https://doi.org/10.1021/acsomega.3c02558. doi:10.1021/acsomega.3c02558.

[7] L. Sendra, A. Beardo, P. Torres, J. Bafaluy, F. X. Alvarez, J. Camacho, Derivation of a hydrodynamic heat equation from the phonon boltzmann equation for general semiconductors, Phys. Rev. B 103 (2021) L140301. URL: https://link.aps.org/doi/10.1103/PhysRevB.103.L140301. doi:10.1103/PhysRevB.103.L140301.
